# Supplementary material for: On the Computation of Form Factors in Massless QCD with Finite Master Integrals
Source: arXiv:1510.06758 ancillary file (2016-08-28)
Supplement: Supplementary file 1 [file Dictionary.pdf]

$$\begin{aligned}
& \text{INT}[\text{"A1diminc2"}, 2, 3, 4, 0, \{2, 2, 0\}] &= \text{Diagram 1} & (6-2\epsilon) \\
& \text{INT}[\text{"A2diminc2"}, 4, 15, 8, 0, \{2, 2, 2, 2, 0, 0, 0\}] &= \text{Diagram 2} & (6-2\epsilon) \\
& \text{INT}[\text{"A2diminc4"}, 3, 22, 9, 0, \{0, 3, 3, 0, 3, 0, 0\}] &= \text{Diagram 3} & (8-2\epsilon) \\
& & & (10-2\epsilon) \\
& \text{INT}[\text{"A2diminc6"}, 4, 58, 12, 0, \{0, 3, 0, 3, 3, 3, 0\}] &= \text{Diagram 4} & (8-2\epsilon) \\
& \text{INT}[\text{"B2diminc4"}, 6, 63, 10, 0, \{2, 2, 2, 2, 1, 1, 0\}] &= \text{Diagram 5} & (10-2\epsilon) \\
& \text{INT}[\text{"A3diminc6"}, 4, 172, 16, 0, \{0, 0, 4, 4, 0, 4, 0, 4, 0, 0, 0, 0\}] &= \text{Diagram 6} & (8-2\epsilon) \\
& \text{INT}[\text{"A3diminc4"}, 5, 662, 15, 0, \{0, 3, 3, 0, 3, 0, 0, 3, 0, 3, 0, 0\}] &= \text{Diagram 7} & (6-2\epsilon) \\
& \text{INT}[\text{"A3diminc2"}, 5, 158, 10, 0, \{0, 2, 2, 2, 2, 0, 0, 2, 0, 0, 0, 0\}] &= \text{Diagram 8} & (10-2\epsilon) \\
& \text{INT}[\text{"A3diminc6"}, 5, 412, 16, 0, \{0, 0, 4, 3, 4, 0, 0, 2, 3, 0, 0, 0\}] &= \text{Diagram 9} & (8-2\epsilon) \\
& \text{INT}[\text{"A3diminc4"}, 5, 433, 13, 0, \{2, 0, 0, 0, 3, 3, 0, 2, 3, 0, 0, 0\}] &= \text{Diagram 10} & (8-2\epsilon)
\end{aligned}$$

$$\text{INT}[\text{"A3diminc2"}, 6, 2695, 12, 0, \{2, 2, 2, 0, 0, 0, 0, 2, 0, 2, 0, 2\}] = \text{Diagram 1}$$

$(6-2\epsilon)$   
 $(10-2\epsilon)$

$$\text{INT}[\text{"A3diminc6"}, 6, 1683, 20, 0, \{3, 4, 0, 0, 3, 0, 0, 3, 0, 4, 3, 0\}] = \text{Diagram 2}$$

$$\text{INT}[\text{"A3diminc4"}, 6, 691, 14, 0, \{2, 2, 0, 0, 3, 3, 0, 2, 0, 2, 0, 0\}] = \text{Diagram 3}$$

$(8-2\epsilon)$   
 $(10-2\epsilon)$

$$\text{INT}[\text{"A3diminc6"}, 6, 1433, 16, 0, \{2, 0, 0, 3, 3, 0, 0, 2, 3, 0, 3, 0\}] = \text{Diagram 4}$$

$(6-2\epsilon)$

$$\text{INT}[\text{"A3diminc2"}, 6, 429, 10, 0, \{1, 0, 2, 2, 0, 2, 0, 2, 1, 0, 0, 0\}] = \text{Diagram 5}$$

$(6-2\epsilon)$

$$\text{INT}[\text{"A3diminc2"}, 6, 444, 10, 0, \{0, 0, 2, 2, 1, 2, 0, 2, 1, 0, 0, 0\}] = \text{Diagram 6}$$

$(6-2\epsilon)$

$$\text{INT}[\text{"B3diminc2"}, 7, 1770, 10, 0, \{0, 2, 0, 1, 0, 2, 1, 1, 0, 1, 2, 0\}] = \text{Diagram 7}$$

$(6-2\epsilon)$

$$\text{INT}[\text{"B3diminc2"}, 7, 1780, 10, 0, \{0, 0, 1, 0, 2, 2, 1, 1, 0, 2, 1, 0\}] = \text{Diagram 8}$$

$(8-2\epsilon)$

$$\text{INT}[\text{"B3diminc4"}, 7, 1766, 13, 0, \{0, 2, 2, 0, 0, 3, 2, 1, 0, 2, 1, 0\}] = \text{Diagram 9}$$

$$\begin{aligned}
& \text{INT}[\text{"A3diminc2"}, 7, 758, 10, 0, \{0, 2, 2, 0, 2, 1, 1, 1, 0, 1, 0, 0\}] = \text{Diagram} \quad (6-2\epsilon) \\
& \text{INT}[\text{"B3"}, 7, 1722, 7, 0, \{0, 1, 0, 1, 1, 1, 0, 1, 0, 1, 1, 0\}] = \text{Diagram} \quad (4-2\epsilon) \\
& \text{INT}[\text{"C3diminc4"}, 8, 2959, 16, 0, \{2, 2, 3, 1, 0, 0, 0, 2, 1, 2, 0, 3\}] = \text{Diagram} \quad (8-2\epsilon) \\
& \text{INT}[\text{"B3"}, 8, 2750, 8, 0, \{0, 1, 1, 1, 1, 1, 0, 1, 0, 1, 0, 1\}] = \text{Diagram} \quad (4-2\epsilon) \\
& \text{INT}[\text{"B3diminc2"}, 8, 1662, 10, 0, \{0, 1, 1, 2, 1, 1, 1, 0, 0, 2, 1, 0\}] = \text{Diagram} \quad (6-2\epsilon) \\
& \text{INT}[\text{"A3diminc2"}, 9, 1790, 10, 0, \{0, 1, 1, 1, 2, 1, 1, 1, 0, 1, 1, 0\}] = \text{Diagram} \quad (6-2\epsilon) \\
& \text{INT}[\text{"B3diminc2"}, 9, 1790, 10, 0, \{0, 1, 1, 2, 1, 1, 1, 1, 0, 1, 1, 0\}] = \text{Diagram} \quad (6-2\epsilon) \\
& \text{INT}[\text{"C3diminc2"}, 9, 1015, 10, 0, \{1, 1, 1, 0, 1, 2, 1, 1, 1, 1, 0, 0\}] = \text{Diagram} \quad (6-2\epsilon)
\end{aligned}$$
